# Supplementary material for: Graph Neural Network Policies and Imitation Learning for Multi-Domain Task-Oriented Dialogues
Source: arXiv:2210.05252 source file (2022-10-11)
Supplement: Supplementary file 1 [file interface.tex]

\subsection{Interface for Human Evaluation}

We used human annotators for our final dialogue system evaluation. All the participants are colleagues of our research team. They were invited by email to participate in the evaluation freely. All instructions were communicated by email and recalled on the annotation interface. The interface was developed internally by the team. Screenshots of all information provided to the participants are presented in
%Figure~\ref{fig:interface1}, 
Figure~\ref{fig:interface2} and Figure~\ref{fig:interface3}.

%\begin{figure}[ht!]
%  \begin{center}
%    \includegraphics[width=0.9\linewidth]{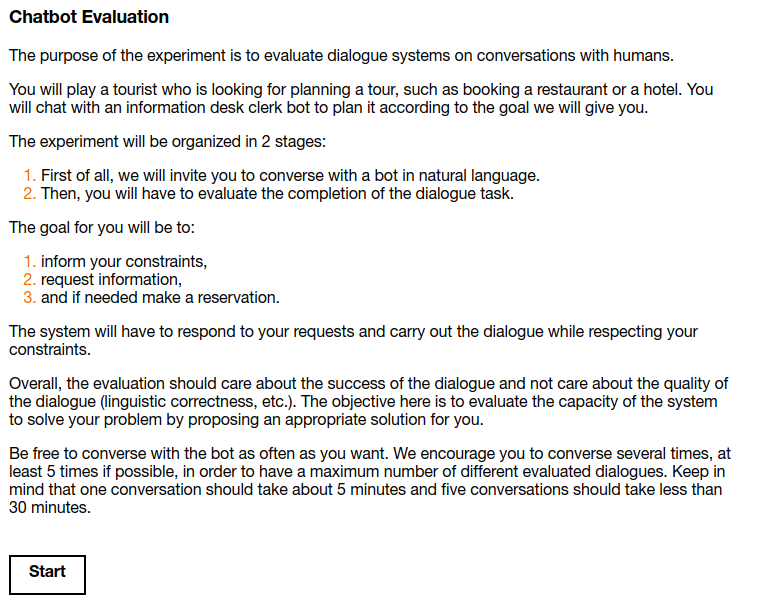}
%  \end{center}
%  \caption{Interface screen presenting the chatbot evaluation.}
%  \label{fig:interface1}
%\end{figure}

\begin{figure}[ht!]
  \begin{center}
    \includegraphics[width=0.9\linewidth]{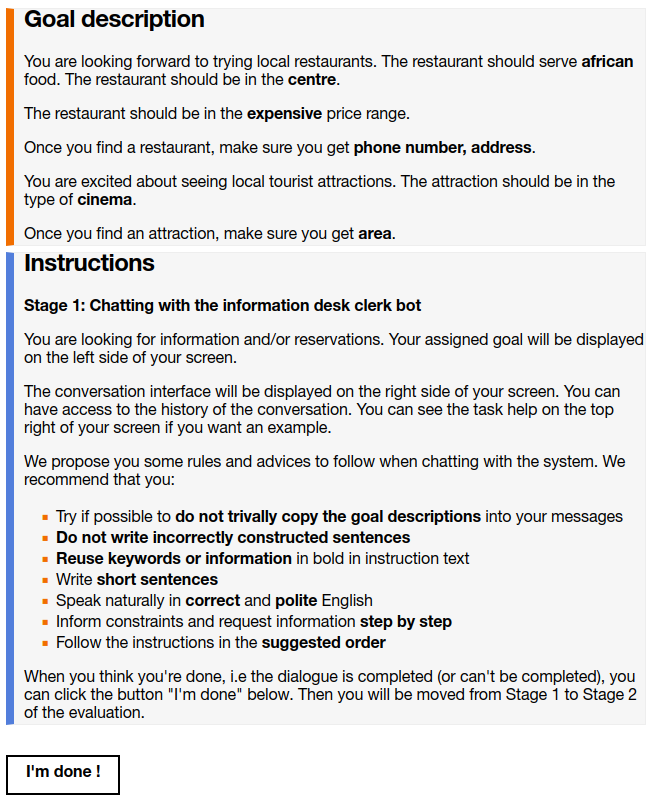}
  \end{center}
  \caption{Interface screen presenting the goal description for the current dialogue and the instructions to follow.}
  \label{fig:interface2}
\end{figure}

\begin{figure}[ht!]
  \begin{center}
    \includegraphics[width=0.9\linewidth]{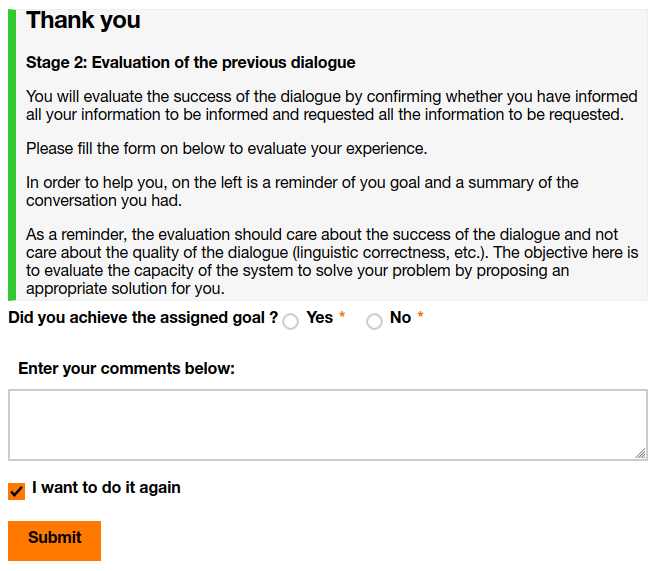}
  \end{center}
  \caption{Interface screen presenting the instructions of the evaluation stage.}
  \label{fig:interface3}
\end{figure}
